# Supplementary material for: Generalization of the Wall Theorem to Out-of-equilibrium Conditions
Source: arXiv:1906.06264 source file (2019-06-14)
Supplement: Supplementary file 1 [file supplmat.pdf]

# SUPPLEMENTARY MATERIAL

## I. DEDUCTION OF $s = \mathrm{in}$ CASE:

We consider particles in the skin $\partial\mathcal{A}^\epsilon$ going in the in direction with normal momentum in a small interval $(p_z, p_z + \Delta p_z)$, in the negative domain. The normal outward versor for any point in $\partial\mathcal{A}^\epsilon$ is $\hat{z} = \hat{\mathbf{n}}_{\mathrm{out}}$. Each particle in $\partial\mathcal{A}^\epsilon$ has a constant velocity to a good approximation. This approximation becomes better for a progressively smaller $\epsilon$. The number of particles in $\partial\mathcal{A}^\epsilon$ that have fluxed from the wall to $\partial\mathcal{A}^\epsilon$ per unit time, having normal momentum between $p_z$ and $p_z + \Delta p_z$ along an small time interval $\tau$ is given by

$$\frac{1}{\tau}\iint\int_0^{-\tau p_z/m} \rho_{\mathrm{in}}\left(\mathbf{r},\mathbf{p}\right) J_{\mathbf{r}} J_{\mathbf{p}} dz\, \Delta p_z d\mathbf{r}_{\bar{z}} d\mathbf{p}_{\bar{z}}\ , \tag{1}$$

where $p_z$ is negative and we assume $\epsilon > -\tau p_z/m$. We write $d\mathbf{r} = J_{\mathbf{r}} dz d\mathbf{r}_{\bar{z}}$ and $d\mathbf{p} = J_{\mathbf{p}} dp_z d\mathbf{p}_{\bar{z}}$, with $J$ the jacobian, to explicitly separate the differential in the $z$ direction both, in space and momentum, from the other directions. For example, if we were dealing with cartesian coordinates and a planar wall at $z = 0$ we have $d\mathbf{r}_{\bar{z}} = dxdy$, evenmore, for a cylindrical channel we should replace in Eq. (1) $dz = dr$ and $d\mathbf{r}_{\bar{z}} = d\theta dz$ (the same applies in momentum space). The mean flux of a quantity $Y\left(\mathbf{r},\mathbf{p}\right)$ is then

$$-\frac{1}{\tau}\iint\int_0^{-\tau p_z/m} Y \rho_{\mathrm{in}}\left(\mathbf{r},\mathbf{p}\right) J_{\mathbf{r}} J_{\mathbf{p}} dz\, \Delta p_z d\mathbf{r}_{\bar{z}} d\mathbf{p}_{\bar{z}}\ . \tag{2}$$

Specifically, this is the flux of $Y$ from the wall towards the fluid exerted by particles with normal momentum in the range $(p_z, p_z + \Delta p_z)$. An extra factor $(-1)$ was included in Eq. (2) to express that particles are leaving the wall. Now we do the integral in $dz$, after that take the limits $\lim\limits_{\epsilon\to 0}\lim\limits_{\tau\to 0}$, and finally replace $\Delta p_z$ with $dp_z$ to integrate in $dp_z$. All these steps transform Eq. (2) to

$$\iint\int \frac{\mathbf{p}\cdot\hat{\mathbf{n}}}{m} Y_w\left(\mathbf{p}\right) \rho_{w,\mathrm{in}}\left(\mathbf{p}\right) \left(J_{\mathbf{r}} J_{\mathbf{p}}\right)_w dp_n d\mathbf{r}_{\bar{n}} d\mathbf{p}_{\bar{n}}\ ,$$

which is identical to the Eq. (10) in the manuscript. This can be casted to a volumetric integral in space by including the $\delta\left(|\partial\mathcal{A} - \mathbf{r}|\right)$ term, and using the $s$-subsystem notation one reaches $j_{w,s}(Y)$, at Eq. (11) of the manuscript.

Those integrals over the volume $\mathcal{A}$ with a term $\delta\left(|\partial\mathcal{A} - \mathbf{r}|\right)$ in the integrand are easily transformed to surface integrals over $\partial\mathcal{A}$, as $\int Z\, \delta\left(|\partial\mathcal{A} - \mathbf{r}|\right) d\mathbf{r} = \int Z\, d\mathrm{S}$. Therefore,

$$\rho_{w,s} = A^{-1}\iint \rho_s\left(\mathbf{r},\mathbf{p}\right) d\mathbf{p} d\mathrm{S}\ , \tag{3}$$

$$\left[X\right]_s \rho_{w,s} = A^{-1}\iint X \rho_s\left(\mathbf{r},\mathbf{p}\right) d\mathbf{p} d\mathrm{S}\ , \tag{4}$$

$$P_{w,s} = A^{-1}\iint \frac{\left(\mathbf{p}\cdot\hat{\mathbf{n}}\right)^2}{m} \rho_s\left(\mathbf{r},\mathbf{p}\right) d\mathbf{p} d\mathrm{S}\ . \tag{5}$$

## II. SIMULATION DETAILS

### A. Reduced Units

For the event-driven molecular-dynamics simulations we use reduced units, defined in terms of the parameters of the square-well potential. Lengths are measured in units of $\sigma$, energies in units of $\varepsilon$ and masses in terms of $m = 1$. The boltzmann constant is also set to unity: $k = 1$. From this the unit of time $\tau$ can be defined as $\tau = \left(m\sigma^2/\varepsilon\right)^{1/2}$, the unit pressure as $\varepsilon/\sigma^3$ and the number density as $\sigma^{-3}$.

### B. External driving

As the event-driven simulation has no explicit forces, unlike continuum-potential molecular-dynamics simulations, the external forces of the system were applied by changing the momentum of particles at a regular interval in particle-interaction events, by adding a constant velocity $v_0$ on each particle in the axial $z$-direction. We applied this external constant velocity each five events. The external force can then, be calculated as $F = mv_0 n_f/\tau_0$, where $\tau_0$ is the total time of simulation and $n_f$ the number of events with $v_0$ application.

### C. Wall contact quantities

We present here the formulas used to measure different relevant quantities in the EDMD simulation. The density on the wall for $s = \text{in}, \text{out}$ is

$$\rho_{w,s} = \frac{1}{\tau_0 dr\, A} \sum_{\text{events}} \frac{dr}{|v_{r,s}|}\,, \tag{6}$$

where the sum runs over the wall events. The total density is $\rho_w = \sum_s \rho_{w,s}$. In Eq. (6) the term $1/|v_{r,s}|$ is a kinematic weight, that takes into account the time that the particle stays at an infinitesimal control volume $dr\,A$ next to the wall, before or after the collision. $dr$, written explicitely for clarity, drops out in Eq. 6, and it will be omitted in the following relations.

The temperature on the wall following a direction $d$ (with $d = r, \theta$) is

$$T^{(d)}_{w,s} = \frac{m}{\tau_0 A k \rho_{w,s}} \sum_{events} \frac{v^2_{d,s}}{|v_{r,s}|}\,. \tag{7}$$

The overall temperature in direction $d$ is calculated as $T^{(d)}_w = \rho_w^{-1} \sum_s T^{(d)}_{w,s}\rho_{w,s}$. In the case of pressure it is

$$P_{w,s} = \frac{m}{\tau_0 A} \sum_{events} |v_{r,s}|\,, \tag{8}$$

with $P_w = \sum_s P_{w,s}$.

Profiles in Fig. 2 were obtained with the usual scheme of binning for the MD box in concentric cylinders of thickness $\Delta r = 0.02002\sigma$, giving rise to 500 points in the profiles of density, velocity and temperature (Fig. 2 in the paper). Properties measured on the wall were compared with the profiles to cross-check our results.

## III. PRESSURE VS. DENSITY

We complement here the results of NEWT presented in Fig. 1 of the paper. We study the evolution of $P_w$ vs. $\rho_w$ at constant wall temperature and liquid number density $\rho_0 = 0.6$. The change of the quantities on the wall are due solely to the increase of the liquid driving. In Fig. 1 we show the "isotherm" of nanoconfined steady-state flow. As $F$ increases, both density and pressure on the wall, increase also. $P_w$ (red line) and $\rho_w T^{(r)}_w$ (open circles) are the mean values, as obtained from simulation averages. They present an excellent agreement for the whole range of densities. Additionally, we provide two alternative trial expressions to approximate the pressure, based on two characteristic temperatures. The curve which results from applying the equilibrium WT, i.e. using the wall temperature, is shown in blue diamonds. An alternative approach that uses $T^{(\theta)}_w$ as a local measure of the fluid temperature at the wall is shown in green squares. Interestingly, the curves are very close to the correct NEWT, albeit the differences are evident at larger wall densities. The equilibrium WT works reasonable well up to $\rho_w \sim 0.7$ for these particular conditions. The expression with $T^{(\theta)}$ gives pretty good results up to $\rho_w \sim 1.5$. The knowledge of the NEWT and the WT allow for a precise determination of the conditions at which non-equilibrium effects start to be apreciable at the wall.

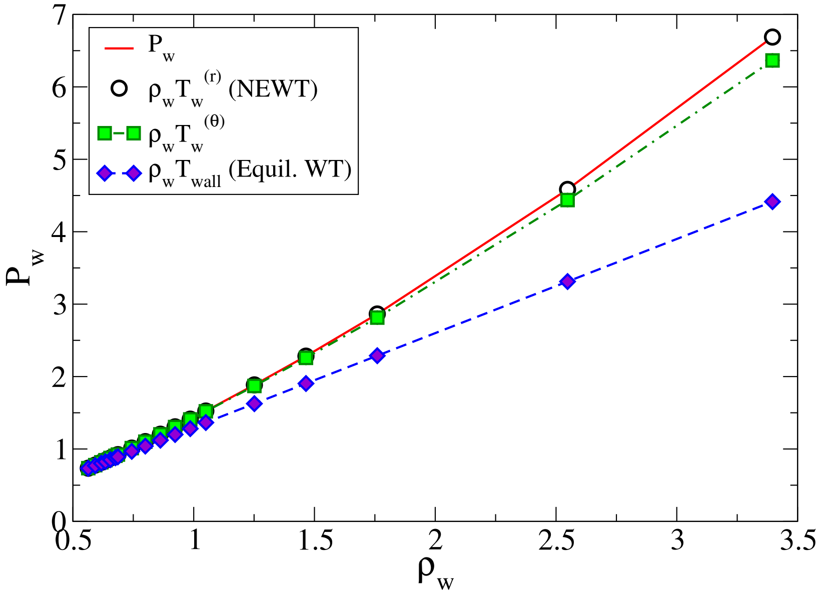


Figure 1. The red line shows the pressure and the black open circles $\rho_w T^{(r)}$, which should be the same following the NEWT expression. The blue curve displays the equilibrium Wall theorem, that uses the wall temperature. In green, we present the same relationship, but using the temperature calculated from the angular variable $\theta$. For close-to-equilibrium conditions the three definitions of temperature give reasonable good results. The expression with $T^{(\theta)}$ continues to give reasonable results for higher drivings. At strong out-of-equilibrium conditions, the differences with the NEWT are appreciable.
